# Supplementary material for: Exploring the formation of gold/silver nanoalloys with gas-phase synthesis and machine-learning assisted simulations
Source: arXiv:2401.05106 source file (2024-01-10)
Supplement: Supplementary file 1 [file SI.pdf]

# Exploring the formation of gold/silver nanalloys with gas-phase synthesis and machine-learning assisted simulations Supplementary information

Quentin Gromoff,[1] Patrizio Benzo,[1] Wissam A. Saidi,[2,3] Christopher M. Andolina,[2,3] Marie-José Casanove,[1] Teresa Hungria,[4] Sophie Barre,[1] Magali Benoit,[1] and Julien Lam[1,5,*]

[1] *CEMES, CNRS and Université de Toulouse, 29 rue Jeanne Marvig, 31055 Toulouse Cedex, France*
[2] *National Energy Technology Laboratory, United States Department of Energy, Pittsburgh, PA 15236, USA*
[3] *Department of Mechanical Engineering and Materials Science, University of Pittsburgh, Pittsburgh, PA 15261, USA*
[4] *Centre de MicroCaractérisation Raimond Castaing, Université de Toulouse, 3 rue Caroline Aigle, F-31400 Toulouse, France*
[5] *Univ. Lille, CNRS, INRA, ENSCL, UMR 8207, UMET, Unité Matériaux et Transformations, F 59000 Lille, France*

* julien.lam@cnrs.fr

## A. EVALUATING THE ACCURACY OF A DEEP NEURAL NETWORK POTENTIAL (DNP) FOR AG-AU ALLOYS

In addition to Andolina et al.'s[1] validation tests, we tested the potential on three bulk alloys: $Au_{0.25}Ag_{0.75}$, $Au_{0.5}Ag_{0.5}$ and $Au_{0.75}Ag_{0.25}$. We evaluated bulk and surface properties. Our results show errors less than 1% for structural properties, and less than to 20% for mechanical properties and surface formation energies (Fig. 1) which are much more challenging to compute with accuracy.

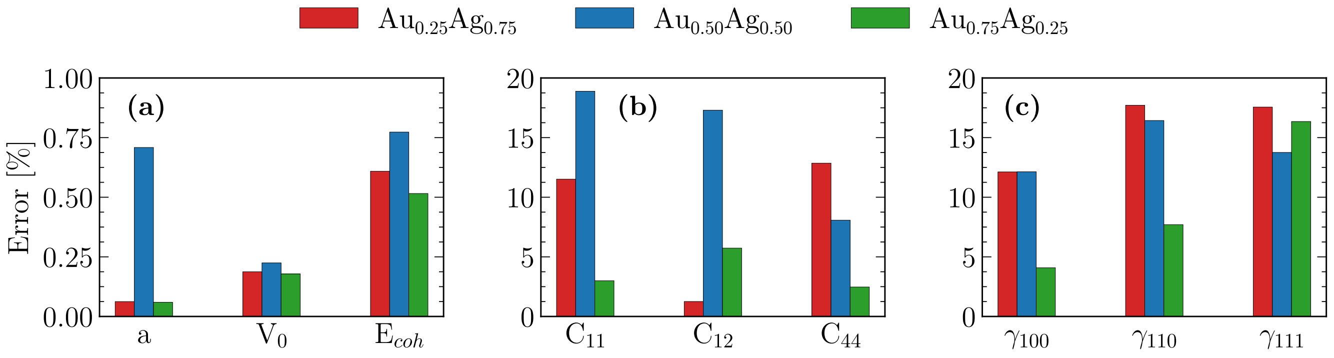


FIG. 1. (a) Lattice constant $a$, lattice volume per atom $V_0$ and cohesive energy $E_{coh}$. (b) Elastic constants $C_{11}$, $C_{12}$, and $C_{44}$. (c) Surface formation energies for (100), (110), and (111) surfaces.

Secondly, we tested amorphous structures. For this purpose, we applied the following procedure:

1. MD simulations were performed at 2000 K on supercells of $Au_{0.25}Ag_{0.75}$, $Au_{0.5}Ag_{0.5}$, and $Au_{0.75}Ag_{0.25}$ ordered alloys.
2. Ten snapshots were selected from the 2000 K MD trajectories to compute the forces using DFT.
3. The liquid structures obtained from the MD simulations were relaxed at 0K using the DNP.
4. After step 3, each structure was further relaxed using DFT.

The resulting changes after the final DFT relaxation are illustrated by the example shown in Fig. 2.

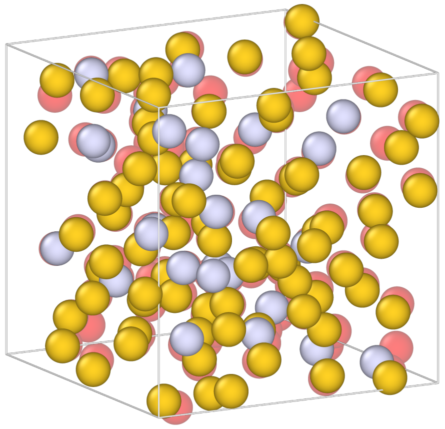

FIG. 2. Snapshot of a 108 atoms $Au_{0.75}Ag_{0.25}$ system after the quench and relaxation with DFT. Yellow (Au) and grey (Ag) atoms correspond to the structure after step 3. Red atoms correspond to the structure after step 4.

In Figure 3(a), the atomic displacements after the DFT relaxation (step 4) are presented: they show a tight distribution with a peak at 0.1 Å and an average displacement of MSD = 0.6 Å, demonstrating the validity of the DNP for disordered structures. In Figure 3(b), the comparison of the forces extracted from the liquid trajectories

and computed using the DNP and DFT are shown: we observe a sharp $y = x$ distribution, with no outliers. The root mean square error (RMSE = $0.07\,\mathrm{eV/Å}$) is within the typical range for machine learning interatomic potentials in the literature.[2]

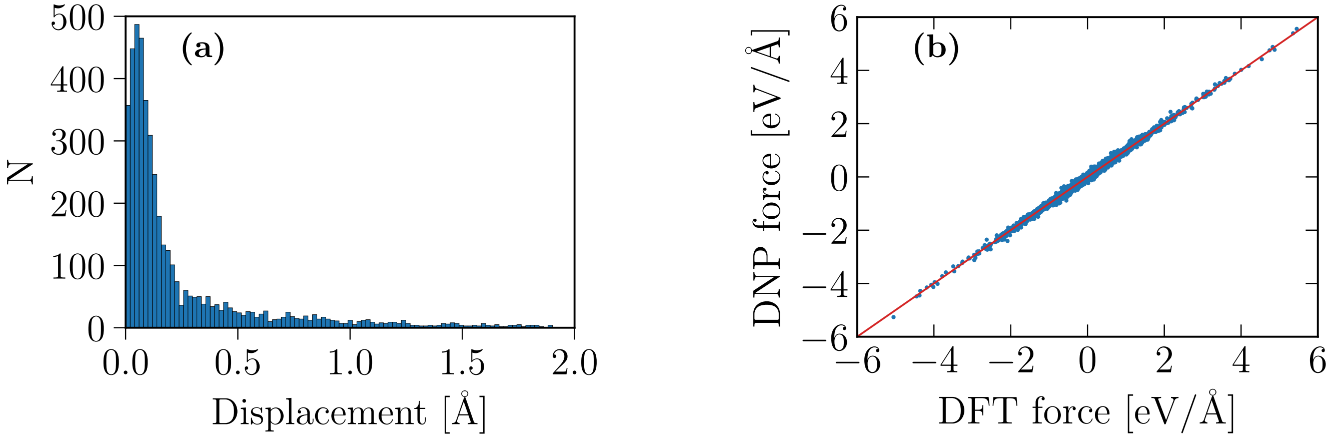


FIG. 3. (a) Distribution of the displacement of atoms between step 3 and step 4 of the procedure. (b) Distribution of the MD versus DFT forces from step 2.

## B. RESULTS OF MONTE-CARLO SIMULATIONS

Monte-Carlo (MC) simulations were conducted on nanoparticles obtained from MD freezing simulations using LAMMPS. The simulations were run for 300 ps while maintaining a constant temperature of 300 K. Additionally, an atom swap operation was performed on all atoms every 100 steps, with a maximum of 10 swaps per atom being allowed. As mentioned in the paper, the shape of the nanoparticles remained stable during MC simulations, but a small change occurred in the $\xi_{surf}$ as shown in Fig. 4. It rose at the beginning of the run, then quickly reached a plateau, for all systems. This suggests a slight increase in gold segregation at the surface of the nanoalloys resulting from the atom swap mechanism. These MC simulations suggest that the gold segregation observed at the end of the freezing MD simulations is not the result of a kinetic pathway but is truly thermodynamically stable.

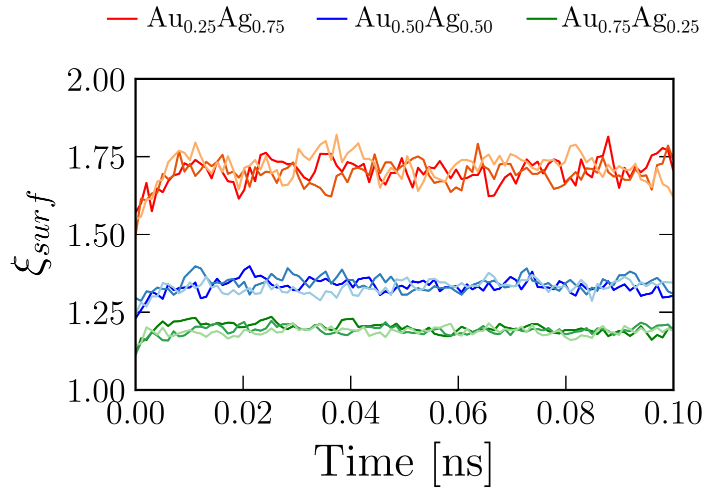


FIG. 4. Evolution of $\xi_{surf}$ in 750 atom nanoparticles over the course of the MC run.

### C. HAADF-STEM OBSERVATION

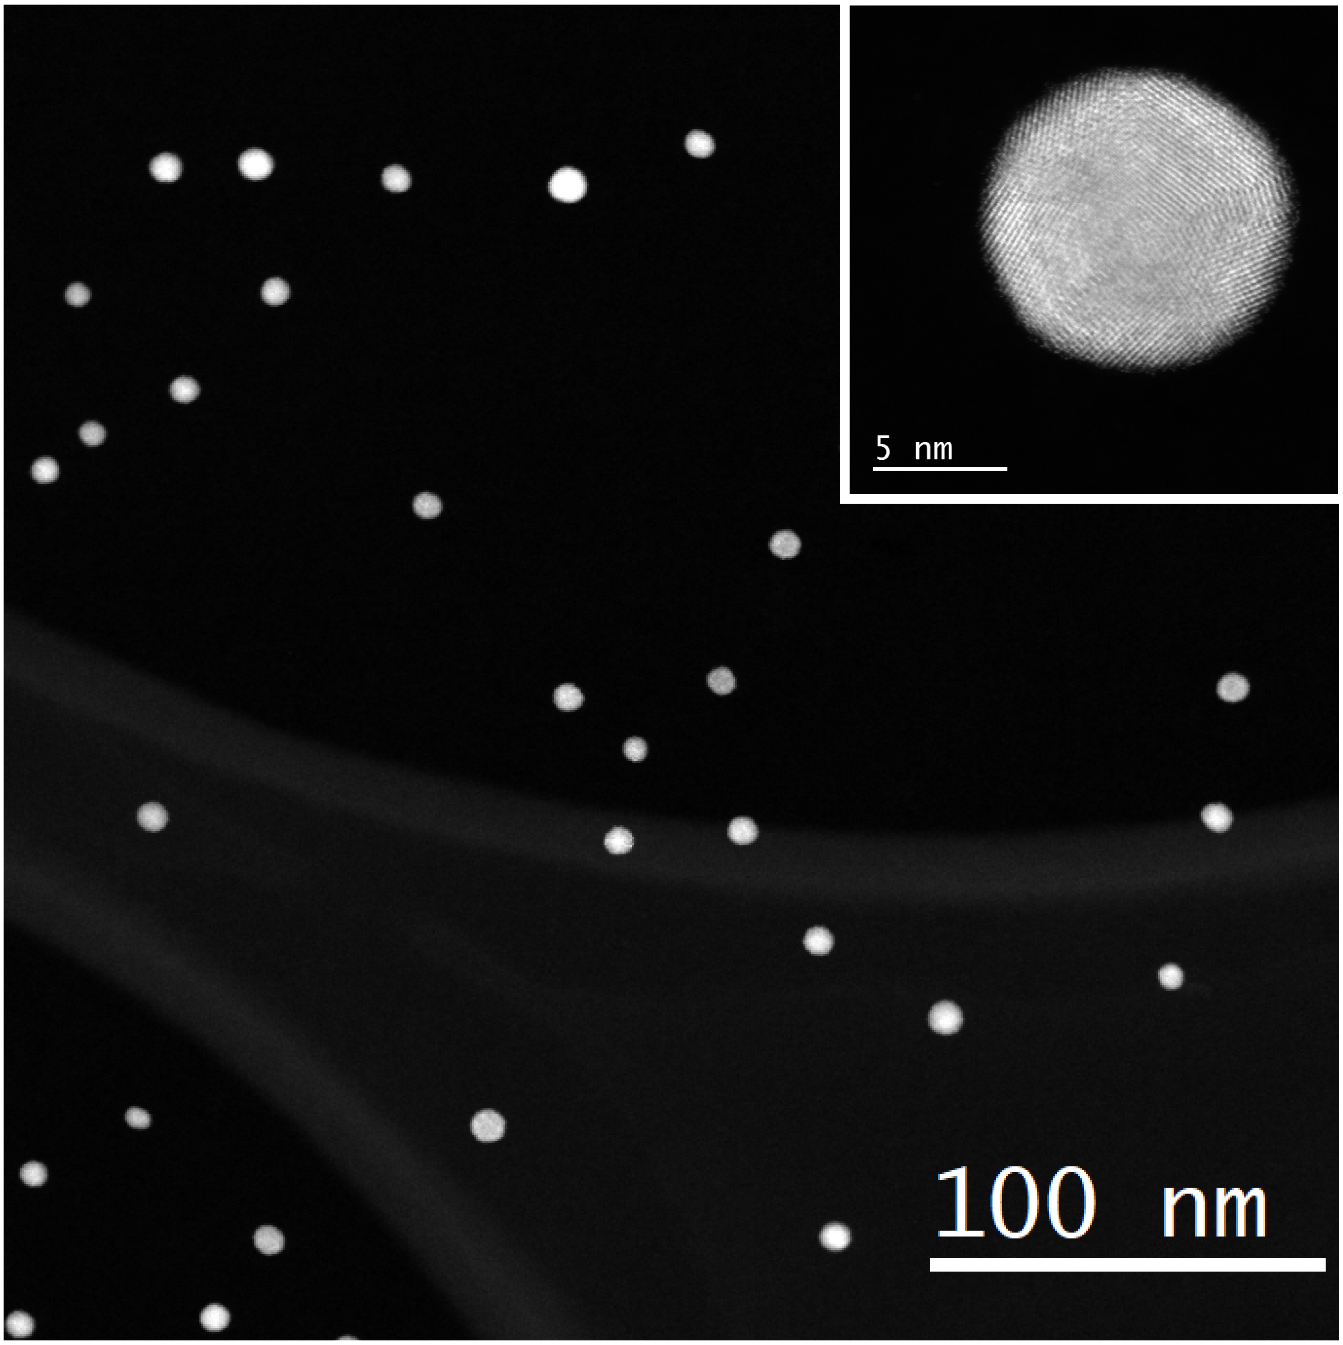


FIG. 5. HAADF-STEM observations of the AuAg nanoparticles synthesized by gas-aggregation magnetron-sputter deposition. The image in inset qualitatively reveal the gold surface segregation in a single nanoparticle (z-contrast).

## D. DENSITY PROFILE OF SIMULATED NANOPARTICLES

The goal of this section was to extract from the simulated nanoparticles a similar information as obtained by EDX measurements in the experiments. For this purpose, we plotted the distribution of the atoms as a function of the distance to the center of mass of the system for both chemical species. We note that with this approach, the integration volume decreases when $r$ decreases which explains that the distribution tends towards 0 for small values of $r$. Despite lacking the clarity of the EDX profiles, it is still possible to compare the distributions of gold and silver in all systems. In particular, the gold segregation is clearly visible through the large peak which correspond to the surface layer.

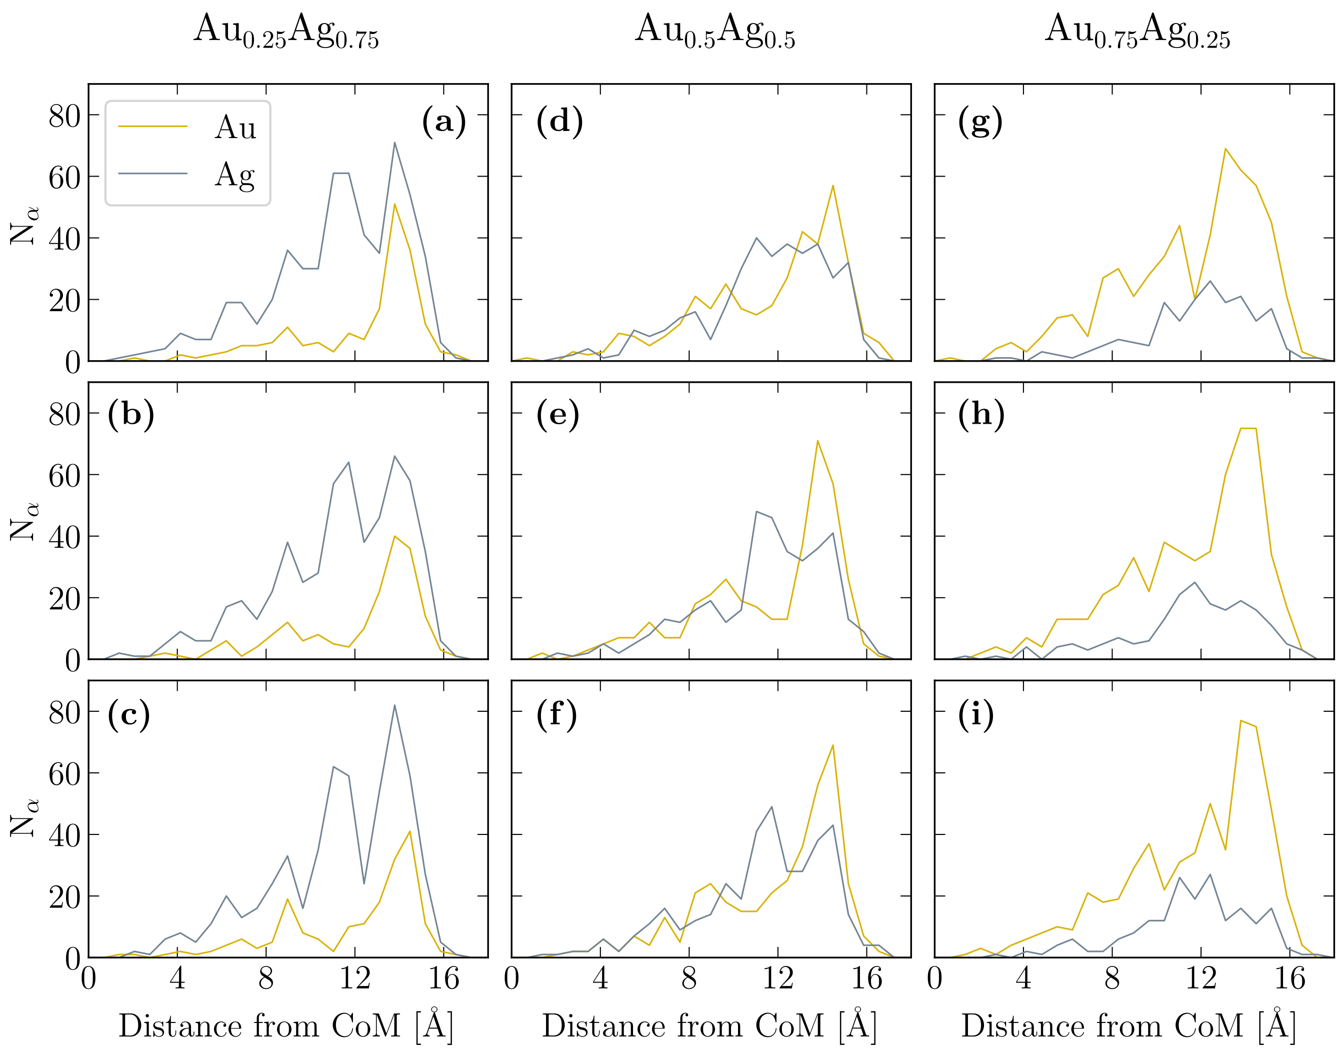


FIG. 6. Distribution of atomic species as a function of distance from the center of mass of the system. The NPs contain 750 atoms, (a,b,c) for $Ag_{0.75}Au_{0.25}$ systems, (d,e,f) for $Ag_{0.50}Au_{0.50}$ systems, (g,h,i) for $Ag_{0.25}Au_{0.75}$ systems.

## E. ADDITIONAL TEMPORAL EVOLUTION OF SIMULATED NANOPARTICLES

Each MD simulation was run three times with different initial conditions. In Fig. 7, we collected the data from all of the 750-atom systems. The trends shown in Fig. 3 of the paper are still valid for the additional simulations. With the exception of one $Au_{0.5}Ag_{0.5}$ particle, the most gold-rich nanoalloys tend to have a low crystalline fraction. In order to make Fig. 7(c) more readable, we have not plotted the data for clusters of less than 50 atoms.

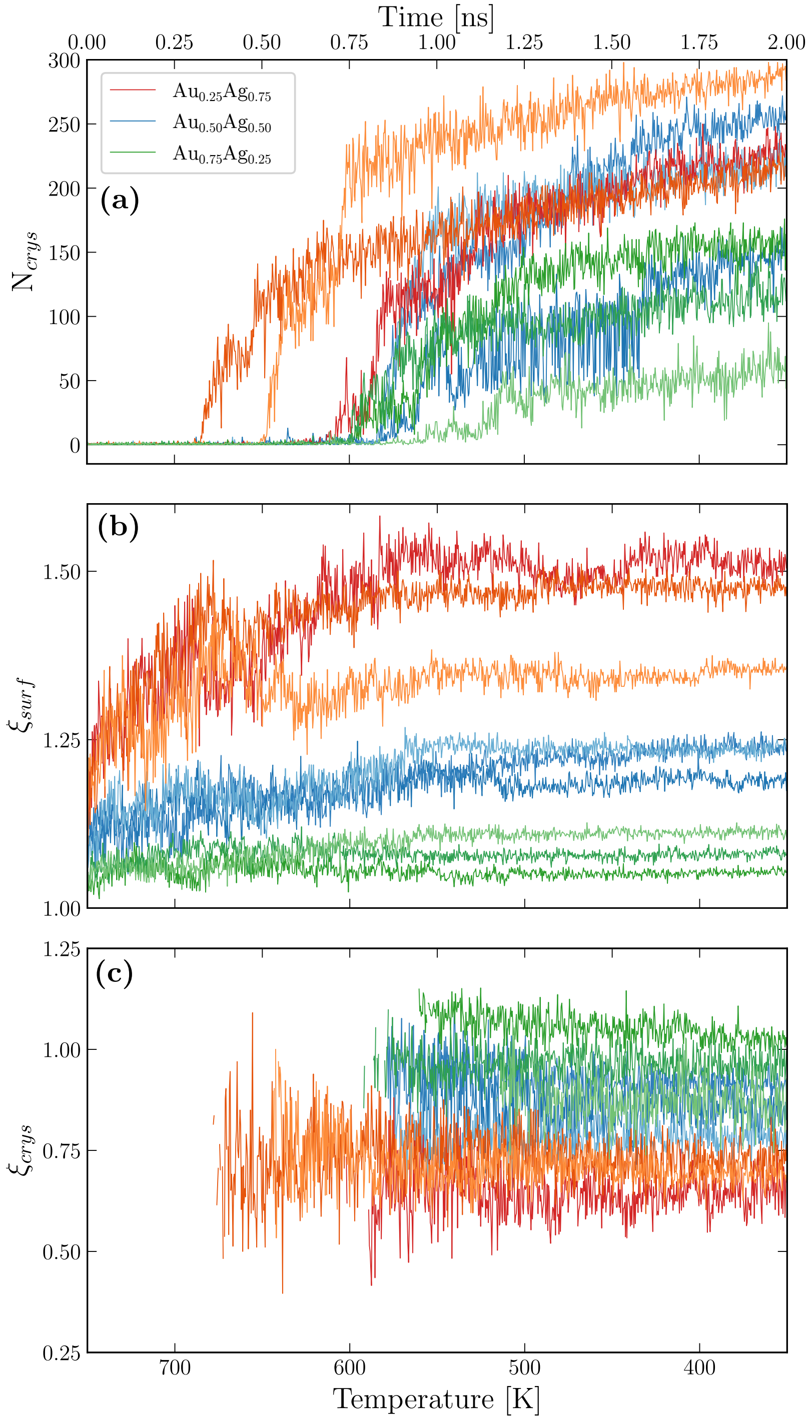


FIG. 7. Additional temporal evolution of $N_{crys}$, $\xi_{surf}$, and $\xi_{crys}$ obtained in MD freezing with nanoparticles of 750 atoms. For each crystal, three runs were carried out with different initial conditions.

## F. STUDY OF THE POSITION OF THE LARGEST CRYSTAL CLUSTER DURING MD SIMULATIONS

In Fig. 8, we show the evolution of the position of the largest crystal cluster at five specific sizes from 10 to 30 atoms. On the y-axis, we calculate the distance between the center of mass of the cluster and that of the whole nanoparticle, divided by the radius of the nanoparticle. Thus, a value greater than 0.5 shows that the cluster is located closer to the surface. Fig. 8(a), (b) and (c) show the results for systems with 250, 500 and 750 atoms, respectively. The most noticeable result is that crystallization begins near the surface of the droplet. We note that surface atoms cannot be classified as part of a crystal cluster due to the algorithm used, which explains why the cluster location can never reach a value of 1.

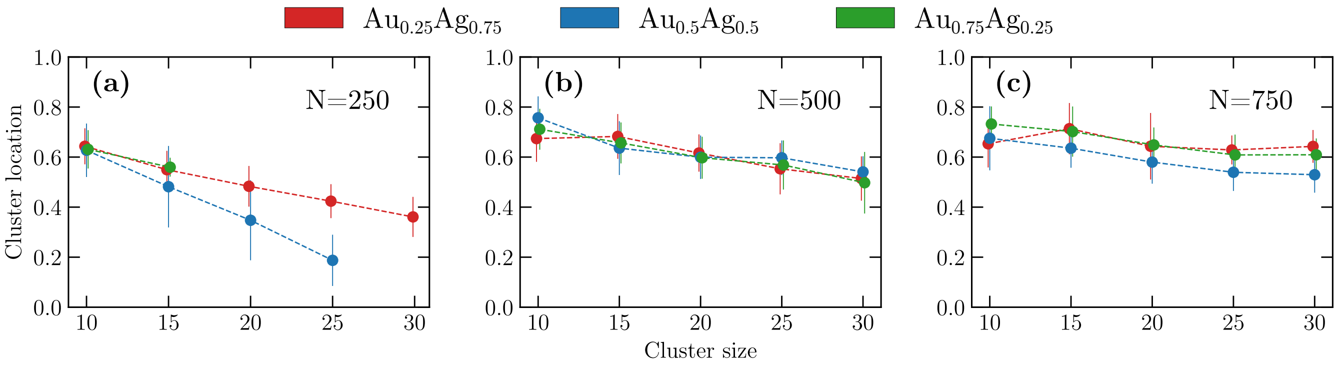


FIG. 8. Evolution of the position of the largest crystal cluster during the MD simulation for three different system sizes.

## G. COORDINATION ANALYSIS OF SIMULATED NANOPARTICLES

Each column in Fig. 9 represents the evolution of the radial distribution function (RDF) for a 750-atom system throughout the freezing simulation. The combined partial distributions are consistent with a solid solution that the Au-Ag alloy is known to form. The transformation from a disordered structure to a more ordered structure can be seen by the increase in the height of the first peak and the appearance of additional secondary peaks at $t = 1\,\mathrm{ns}$ and $t = 2\,\mathrm{ns}$.

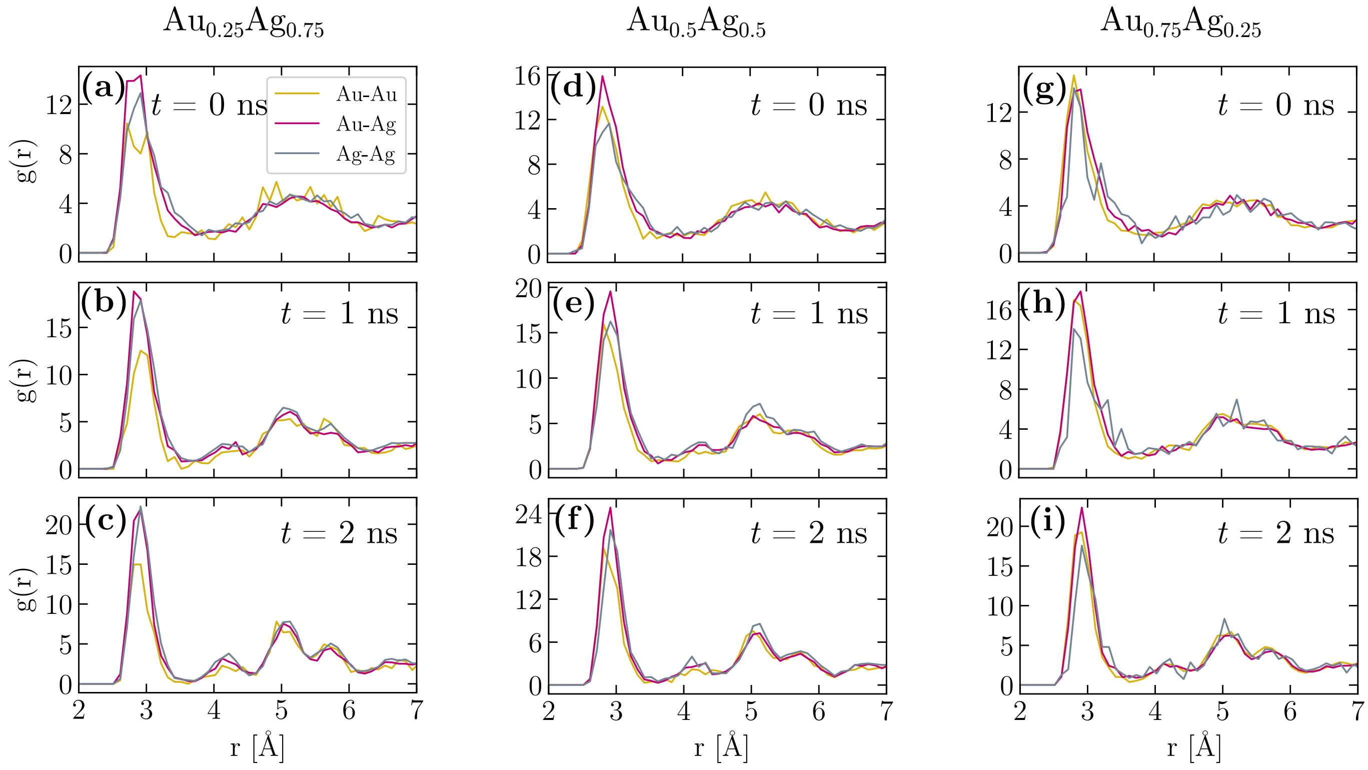


FIG. 9. Partial radial distribution functions RDF for three simulated 750-atoms NPs at different stages of the MD run.


[1] C. M. Andolina, M. Bon, D. Passerone, and W. A. Saidi, J. Phys. Chem. C **125**, 17438 (2021).
[2] Y. Wang, L. Zhang, B. Xu, X. Wang, and H. Wang, Model. Simul. Mater. Sci. Eng. **30**, 025003 (2021).
